# Supplementary material for: Non-Hermitian dislocation modes: Stability and melting across exceptional points
Source: arXiv:2105.05244 ancillary file (2022-07-12)
Supplement: Supplementary file 1 [file NHDisloc_Supplementary.pdf]

# Supplementary Material: Non-Hermitian dislocation modes: Stability and melting across exceptional points

Archisman Panigrahi,<sup>1</sup> Roderich Moessner,<sup>2</sup> and Bitan Roy<sup>3</sup>

<sup>1</sup>*Indian Institute of Science, Bangalore 560012, India*

<sup>2</sup>*Max-Planck-Institut für Physik komplexer Systeme, Nöthnitzer Str. 38, 01187 Dresden, Germany*

<sup>3</sup>*Department of Physics, Lehigh University, Bethlehem, Pennsylvania, 18015, USA*

(Dated: May 11, 2021)

The Supplementary Material contains: (1) anti-unitary particle-hole symmetry of the non-Hermitian Chern insulator (Sec. I), (2) tight-binding model in the presence of dislocation in real space (Sec. II), (3) particle-hole symmetry of the dislocation modes (Sec. III), (4) computation of  $h_x^*$ ,  $h_y^*$ ,  $h_z^*$  (Sec. IV), (5) topological invariant: Chern Number (Sec. V), (6) density profile of dislocation modes in systems with open boundary condition (Sec. VI), and (7) code for numerical calculation (Sec. VII).

## I. ANTI-UNITARY PARTICLE-HOLE SYMMETRY OF THE NON-HERMITIAN CHERN INSULATOR

The operator describing a non-Hermitian (NH) Chern insulator in the presence of generic NH perturbations reads

$$\mathcal{H} = t (\sin k_x \sigma_x + \sin k_y \sigma_y) + [t_0 (\cos k_x + \cos k_y) - m_0] \sigma_z + i (h_0 \sigma_0 + h_x \sigma_x + h_y \sigma_y + h_z \sigma_z). \quad (1)$$

Here  $h_0, h_x, h_y, h_z$  are real numbers,  $\mathbf{k}$  is the momentum, and  $i = \sqrt{-1}$ . In main text we already mentioned the parameter regimes over which the system describes a Chern insulator when  $h_0 = h_x = h_y = h_z = 0$ . As  $h_0 \sigma_0$  only causes an overall shift of the eigenvalue spectra of  $\mathcal{H}$ , we set  $h_0 = 0$  from the outset. In addition, we also set  $t = t_0 = 1$  throughout. In Sec. II, we show the real space implementation of this model on a square lattice in the presence of a dislocation.

Let  $\mathcal{K}$  be the complex conjugation operator, such that  $\mathcal{K}i \rightarrow -i$  and  $\mathcal{K}\mathbf{k} \rightarrow -\mathbf{k}$ . When  $h_z = 0$ , the antiunitary operator  $\Theta = \sigma_x \mathcal{K}$  anticommutes with the operator  $\mathcal{H}$ , i.e.,  $\Theta \mathcal{H} = -\mathcal{H} \Theta$ . Due to this particle-hole symmetry, for each eigenvalue  $\varepsilon$  of  $\mathcal{H}$ , there exists an eigenvalue  $-\varepsilon^*$ . In Sec. III we will discuss the role of the particle-hole symmetry when  $\varepsilon = \varepsilon^*$  (purely real) or  $\varepsilon = -\varepsilon^*$  (purely imaginary). In addition, we will also discuss the role of a pseudo particle-hole symmetry when  $h_x = h_y = 0$ , yielding  $\Theta \mathcal{H} = -\mathcal{H}^\dagger \Theta$ .

## II. TIGHT-BINDING MODEL IN THE PRESENCE OF A DISLOCATION

The above model from Eq. (1) (with  $h_0 = 0$ ) in the presence of a single edge dislocation and generic NH perturbation translates into the following real space non-Hermitian hopping Hamiltonian

$$\begin{aligned} \hat{h}_{\text{real}} = & \left( \left[ \left( \sum_{n_x=1}^{\ell_x-2} \sum_{n_y=1}^{\ell_y-1} + \sum_{n_x=\ell_x+1}^{L_x-1} \sum_{n_y=1}^{\ell_y-1} + \sum_{n_x=1}^{L_x-1} \sum_{n_y=\ell_y}^{L_y} \right) c_{n_x, n_y}^\dagger c_{n_x+1, n_y} \right] \otimes \frac{it\sigma_x + t_0\sigma_z}{2} \right. \\ & + \left\{ \left( \sum_{n_x=1}^{\ell_x-1} \sum_{n_y=1}^{L_y-1} + \sum_{n_x=\ell_x+1}^{L_x} \sum_{n_y=1}^{L_y-1} \right) c_{n_x, n_y}^\dagger c_{n_x, n_y+1} + \sum_{n_y=\ell_y}^{L_y-1} c_{\ell_x, n_y}^\dagger c_{\ell_x, n_y+1} \right\} \otimes \frac{it\sigma_y + t_0\sigma_z}{2} \Big] + H.c. \Big) \\ & + \sum_{j=1}^{L_x L_y - (\ell_y - 1)} c_{j,j}^\dagger c_{j,j} \otimes [-m_0 \sigma_z + ih_x \sigma_x + ih_y \sigma_y + ih_z \sigma_z], \end{aligned} \quad (2)$$

where  $c_{i,j}$  ( $c_{i,j}^\dagger$ ) is the fermion annihilation (creation) operator at site  $(i, j)$ . In this construction, the core of the edge dislocation is located at  $(\ell_x, \ell_y)$  [see Fig. 1 of the main text]. This construction can be generalized to implement a edge dislocation-antidislocation pair with periodic and open boundary conditions.

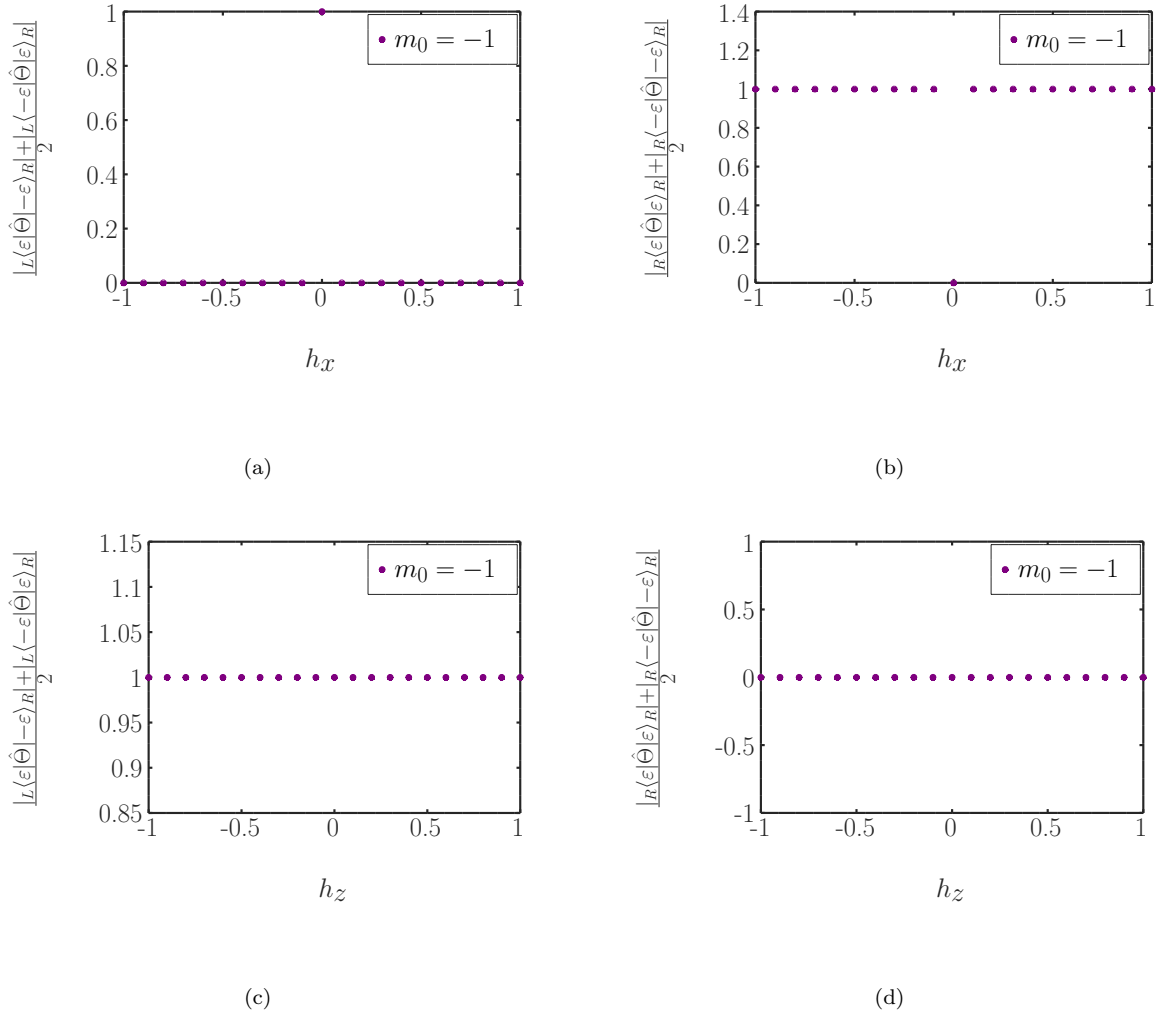

FIG. 1: We fix  $m_0 = -1$ , and plot the inner products (indicated in the  $y$  axis of the respective figures) involving the particle-hole symmetry operator between the two dislocation states, obtained from lattice based numerical simulation. (a) We fix  $h_y = h_z = 0$ . For  $h_x = 0$ , the operator  $\mathcal{H}$  is Hermitian (therefore energy eigenvalues are real) and we get result predicted in Eq. (4) (Note that the indices  $L, R$  have no significance for a Hermitian operator, as in this case). For non-zero  $h_x$ , the energies of the dislocation modes are purely imaginary, and we obtain the results predicted by Eq. (7). We obtain identical result for  $h_x = 0, h_y \neq 0, h_z = 0$ . (b) We fix  $h_y = h_z = 0$ . At  $h_x = 0$ , we get result predicted in Eq. (5). For non-zero  $h_x$ , the energies of the dislocation modes are purely imaginary, and we obtain the results predicted by Eq. (6). We obtain identical result for  $h_x = 0, h_y \neq 0, h_z = 0$ . (c) Here we fix  $h_x = h_y = 0$ . We numerically obtain the result predicted by Eq. (10). (d) We fix  $h_x = h_y = 0$ . We numerically obtain the result predicted by Eq. (11).

### III. DISLOCATION MODES: PARTICLE-HOLE SYMMETRY

Let  $|\varepsilon\rangle_R$  and  $|\varepsilon\rangle_L$  be two right eigenkets corresponding to energy eigenvalues  $+\varepsilon$  and  $-\varepsilon$ . The two dislocation modes form one such set, but the following discussion is more general. We will see how we can obtain one of these states by applying the anti-unitary particle-hole symmetry operator on the other one.

**A. Case I:  $h_z = 0$** 

In this case,  $\mathcal{H}\Theta + \Theta\mathcal{H} = 0$ . Applying this relation on  $|\varepsilon\rangle_R$  from the left, it follows that

$$\mathcal{H}\Theta|\varepsilon\rangle_R = -\varepsilon^*\Theta|\varepsilon\rangle_R. \quad (3)$$

Therefore,  $\Theta|\varepsilon\rangle_R$  is a right eigenket of  $\mathcal{H}$ , with eigenvalue  $-\varepsilon^*$ .

**Sub case:** When  $\varepsilon$  is real,  $\varepsilon = \varepsilon^*$ . Then,  $\Theta|\varepsilon\rangle_R$  is the same as  $|\varepsilon\rangle_R$  up to a phase factor of unit modulus. We must have, for some  $\theta$ ,

$$\Theta|\varepsilon\rangle_R = e^{i\theta}|\varepsilon\rangle_R.$$

Using the antiunitary property of  $\Theta$ , it can be shown that  $\Theta|\varepsilon\rangle_R = e^{i\theta}|\varepsilon\rangle_R$ , with the same  $\theta$ , the value of which depends on the choice of the phases of the eigenstates. Therefore,

$$|_R \langle -\varepsilon | \Theta |\varepsilon\rangle_R | = 1 = |_R \langle \varepsilon | \Theta | -\varepsilon\rangle_R |. \quad (4)$$

Also, due to the biorthogonality relation (i.e.,  $_L \langle \varepsilon_1 | \varepsilon_2 \rangle_R = 0$ , if  $\varepsilon_1 \neq \varepsilon_2$ ),

$$_L \langle \varepsilon | \Theta |\varepsilon\rangle_R = 0 = _L \langle -\varepsilon | \Theta | -\varepsilon\rangle_R. \quad (5)$$

**Note:** Eq. (4) and Eq. (5) hold even for the Hermitian operator  $\mathcal{H}$ , for eigenstates  $|\varepsilon\rangle$  and  $|\varepsilon\rangle$ , the only difference being that the indices  $L, R$  do not have any significance.

**Sub case:** When  $\varepsilon$  is purely imaginary,  $-\varepsilon^* = \varepsilon$ . From Eq. (3), we infer that  $\Theta|\varepsilon\rangle_R$  is same as  $|\varepsilon\rangle_R$ , apart from a phase factor, i.e. for some  $\theta_1$ ,

$$\Theta|\varepsilon\rangle_R = e^{i\theta_1}|\varepsilon\rangle_R.$$

Therefore,

$$|_R \langle \varepsilon | \Theta |\varepsilon\rangle_R | = 1 = |_R \langle -\varepsilon | \Theta | -\varepsilon\rangle_R |. \quad (6)$$

Due to the biorthogonality relation

$$_L \langle -\varepsilon | \Theta |\varepsilon\rangle_R = 0 = _L \langle \varepsilon | \Theta | -\varepsilon\rangle_R. \quad (7)$$

**B. Case II:  $h_z \neq 0$ ,  $h_x = h_y = 0$** 

In this case,  $\mathcal{H} = \sin k_x \sigma_x + \sin k_y \sigma_y + (\cos k_x + \cos k_y - m_0) \sigma_z + i h_z \sigma_z$ . For this operator, it can be shown that

$$\Theta\mathcal{H} = -\mathcal{H}^\dagger\Theta, \quad (8)$$

which we name the pseudo particle-hole symmetry. From the above relation it follows that

$$\mathcal{H}^\dagger\Theta|\varepsilon\rangle_R = -\Theta\mathcal{H}|\varepsilon\rangle_R = -\varepsilon^*\Theta|\varepsilon\rangle_R. \quad (9)$$

Taking Hermitian conjugate of the relation  $_L \langle -\varepsilon | \mathcal{H} = -\varepsilon_L \langle -\varepsilon |$  we get,

$$\mathcal{H}^\dagger|-\varepsilon\rangle_L = -\varepsilon^*|-\varepsilon\rangle_L.$$

From the above relation and Eq. (9), we see that  $\Theta|\varepsilon\rangle_R$  must be equal to  $|\varepsilon\rangle_L$ , up to an overall unimportant phase factor.

$$\Theta|\varepsilon\rangle_R = e^{i\theta_2}|\varepsilon\rangle_L.$$

Therefore,

$$|_L \langle -\varepsilon | \Theta |\varepsilon\rangle_R | = 1 = |_L \langle \varepsilon | \Theta | -\varepsilon\rangle_R |. \quad (10)$$

Due to the biorthogonality relation

$$_R \langle \varepsilon | \Theta |\varepsilon\rangle_R = 0 = _R \langle -\varepsilon | \Theta | -\varepsilon\rangle_R. \quad (11)$$

We numerically diagonalize the operator  $\mathcal{H}$  in the lattice shown in Fig. 1 of the main paper, and the two dislocation modes indeed satisfy these relations (See Fig. 1).

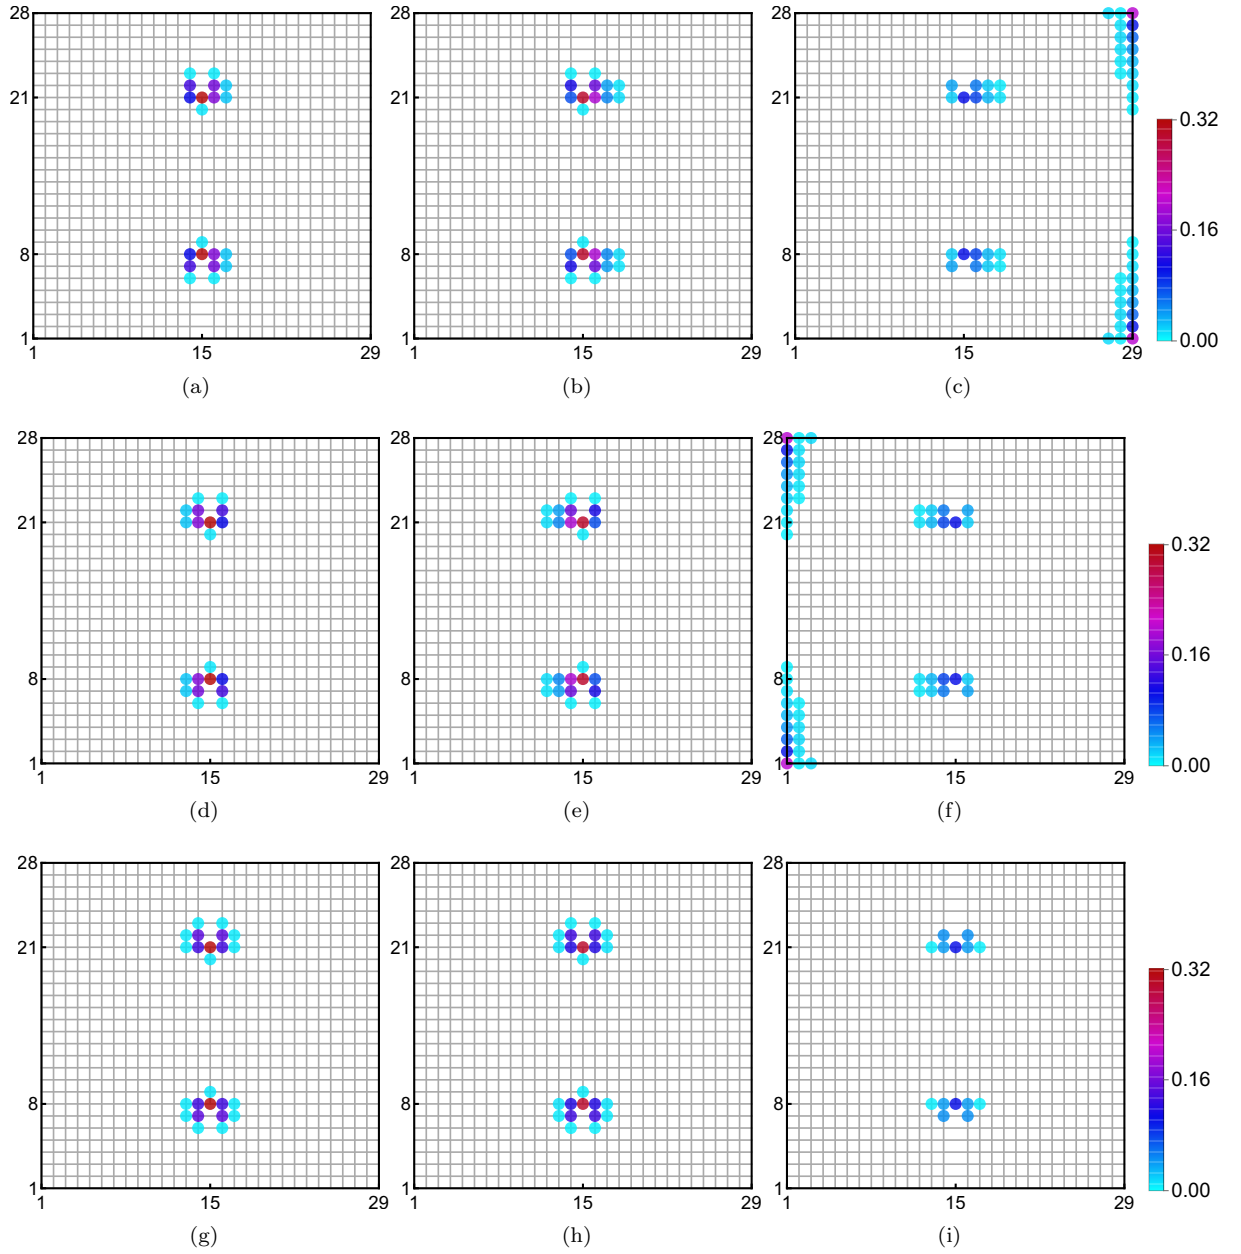

FIG. 2: Spatial profile of the density of the dislocation modes for different values of  $h_x$ , with  $m_0 = -1$ ,  $h_y = h_z = 0$ , under OBC. In (a), (b) and (c), the joint density of the right eigenvectors of the two dislocation modes is plotted for  $h_x = 0.2, 0.4$  and  $0.55$ , respectively. In (d), (e) and (f), the density of the left eigenvectors is plotted for the same set of values of  $h_x$ , and in (g), (h), and (i), the biorthogonal density is plotted. In Fig. (c) and (f), the gradual shift from dislocation modes, to the edge modes (due to skin effect) can be observed.

#### IV. COMPUTATION OF $h_x^*$ , $h_y^*$ , $h_z^*$

The eigenvalues of the NH operator in Eq. (1) are

$$\varepsilon = \pm \sqrt{(\sin k_x + ih_x)^2 + (\sin k_y + ih_y)^2 + (\cos k_x + \cos k_y - m_0 + ih_z)^2} \quad (12)$$

**A. Consider**  $h_x \neq 0, h_y = h_z = 0$ 

In the Argand plane, the eigenvalues of the non-Hermitian operator  $\mathcal{H}$  are distributed like the two wings of a butterfly (See Fig. [3] (a), (b) of the main paper.), and the wings are symmetrically placed about  $y$  axis, define by  $\text{Re}(\varepsilon) = 0$ . As we increase the magnitude of the non-Hermitian parameters, they will gradually come close symmetrically about the  $y$  axis, and join at the origin of the Argand plane (this is the exceptional point) when  $h_x = h_x^*$ . For higher values of  $h_x$ , it is numerically found that there are no dislocation modes, and the system can sustain some purely imaginary energy eigenvalues, irrespective of the presence of dislocation centers. Therefore, we need to check when the system (without dislocation, under PBC) will host states with zero or purely imaginary energy.

**Strategy of the calculation:** When  $\varepsilon$  is purely imaginary,  $\varepsilon^2$  is real and negative. We keep  $m_0$  fixed, and enforce the condition that  $\varepsilon^2$  is real. Then we vary  $k_x, k_y$ , and find the minimum absolute value of  $h_x$  so that  $\varepsilon^2$  still remains negative (so that  $\varepsilon$  can be purely imaginary). That minimum value of  $|h_x|$  is the  $h_x^*$ , which we want to calculate. In other words,  $h_x^*$  is the minimum value of  $h_x$  which allows the system to have zero energy eigenvalues, indicating exceptional points in the Brillouin zone.

**Calculation:** From Eq. (12) we obtain

$$\begin{aligned} \text{Re}(\varepsilon^2) &= 2 + m_0^2 - 2m_0(\cos k_x + \cos k_y) + 2 \cos k_x \cos k_y - h_x^2 \\ \text{Im}(\varepsilon^2) &= 2h_x \sin k_x \end{aligned} \quad (13)$$

For  $\varepsilon^2$  to be real, we need to have

$$\sin k_x = 0 \implies k_x = 0, \pi.$$

Then,  $\cos k_x = \pm 1$ .

Now, we need to find the value of  $k_y$  such that  $\text{Re}(\varepsilon^2)$  is not positive, and  $h_x^2$  is minimum.

$$\begin{aligned} \text{Re}(\varepsilon^2) \leq 0 &\implies 2 + m_0^2 - 2m_0(\cos k_x + \cos k_y) + 2 \cos k_x \cos k_y - h_x^2 \leq 0 \\ &\implies 2 + m_0^2 - 2m_0(\cos k_x + \cos k_y) + 2 \cos k_x \cos k_y \leq h_x^2. \end{aligned} \quad (14)$$

Therefore,

$$\begin{aligned} \min(h_x^2) &= \min [2 + m_0^2 - 2m_0(\cos k_x + \cos k_y) + 2 \cos k_x \cos k_y] \\ h_x^* &= \sqrt{\min [2 + m_0^2 - 2m_0(\cos k_x + \cos k_y) + 2 \cos k_x \cos k_y]}. \end{aligned} \quad (15)$$

Let us focus on the region  $-2 < m_0 < 0$  (the M phase), where dislocation modes are observed.

1. *Case:*  $-1 < m_0 < 0$

Let us consider **sub case I:**  $\cos k_x = +1$ . We then need to minimize the quantity,

$$2 + m_0^2 - 2m_0(1 + \cos k_y) + 2 \cos k_y = 2 + m_0^2 - 2m_0 + \underbrace{2(1 - m_0)}_{\text{positive}} \cos k_y.$$

Since the coefficient of  $\cos k_y$  is positive, the whole quantity is minimum when  $\cos k_y = -1$ . After minimizing with respect to  $k_y$ , the value of the quantity is

$$2 + m_0^2 - 2m_0 - 2(1 - m_0) = m_0^2.$$

Now consider **sub case II:**  $\cos k_x = -1$ . We then need to minimize the quantity

$$2 + m_0^2 - 2m_0(-1 + \cos k_y) - 2 \cos k_y = 2 + m_0^2 + 2m_0 - \underbrace{2(1 + m_0)}_{\text{negative}} \cos k_y.$$

| Interval        | $h_x^* = h_y^*$ | $(k_x, k_y)$                  | Exceptional Point |
|-----------------|-----------------|-------------------------------|-------------------|
| $-1 < m_0 < 0$  | $ m_0 $         | $(\pi, 0)/a$ and $(0, \pi)/a$ | $X$ and $Y$       |
| $-2 < m_0 < -1$ | $ m_0 + 2 $     | $(\pi, \pi)/a$                | $M$               |

TABLE I: Value of  $h_x^* (= h_y^*)$  is tabulated as a function of  $m_0$ . The third column shows the momentum at which the exceptional points first appear in the Brillouin zone. The fourth column shows the corresponding point in the Brillouin zone.

Since the coefficient of  $\cos k_y$  is negative, the whole quantity is minimum when  $\cos k_y = +1$ . After minimizing with respect to  $k_y$ , the value of the quantity is

$$2 + m_0^2 + 2m_0 - 2(1 + m_0) = \boxed{m_0^2}.$$

The minimum value obtained at **sub cases I** and **II** are equal, and  $\boxed{h_x^* = |m_0| = -m_0}$ .

## 2. Case: $-2 < m_0 < -1$

Let us consider **sub case I**:  $\cos k_x = +1$ . We need to minimize the quantity,

$$2 + m_0^2 - 2m_0(1 + \cos k_y) + 2 \cos k_y = 2 + m_0^2 - 2m_0 + \underbrace{2(1 - m_0)}_{\text{positive}} \cos k_y.$$

Since the coefficient of  $\cos k_y$  is positive, the whole quantity is minimum when  $\cos k_y = -1$ . After minimizing with respect to  $k_y$ , the value of the quantity is

$$2 + m_0^2 - 2m_0 - 2(1 - m_0) = \boxed{m_0^2}.$$

Now consider **sub case II**:  $\cos k_x = -1$ . We need to minimize the quantity

$$2 + m_0^2 - 2m_0(-1 + \cos k_y) - 2 \cos k_y = 2 + m_0^2 + 2m_0 \underbrace{-2(1 + m_0)}_{\text{positive}} \cos k_y$$

Since the coefficient of  $\cos k_y$  is positive, the whole quantity is minimum when  $\cos k_y = -1$ . After minimizing with respect to  $k_y$ , the value of the quantity is,

$$2 + m_0^2 + 2m_0 + 2(1 + m_0) = m_0^2 + 4 * m_0 + 4 = \boxed{(m_0 + 2)^2}.$$

**Which sub case to consider?:** In the interval  $1 < m_0 < 2$ ,  $m_0^2 > (m_0 + 2)^2$  [because  $(m_0 + 2)^2 = m_0^2 + \underbrace{4(m_0 + 1)}_{\text{negative}}$ ].

Therefore, the minimum value is obtained at **sub case II**, and  $\boxed{h_x^* = |m_0 + 2|}$ .

This formalism can be extended for any other values of  $m_0$ . The value of  $h_x^*$  is plotted as a function of  $m_0$  in Fig. 2(a) of the main paper.

## B. Consider $h_y \neq 0, h_x = h_z = 0$

Due to the symmetry between  $k_x$  and  $k_y$  in the operator in Eq. (1) (i.e. the  $C_4$  rotation symmetry of the system), the calculation is exactly analogous, and  $h_y^* = h_x^*$  for a given value of  $m_0$ .

## C. Consider $h_z \neq 0, h_x = h_y = 0$

In this case, the wings are **not** symmetrically placed about the  $y$  axis, defined as  $\text{Re}(\varepsilon) = 0$ , and

$$\varepsilon^2 = \sin^2 k_x + \sin^2 k_y + (\cos k_x + \cos k_y - m_0)^2 - h_z^2 + 2ih_z (\cos k_x + \cos k_y - m_0). \quad (16)$$

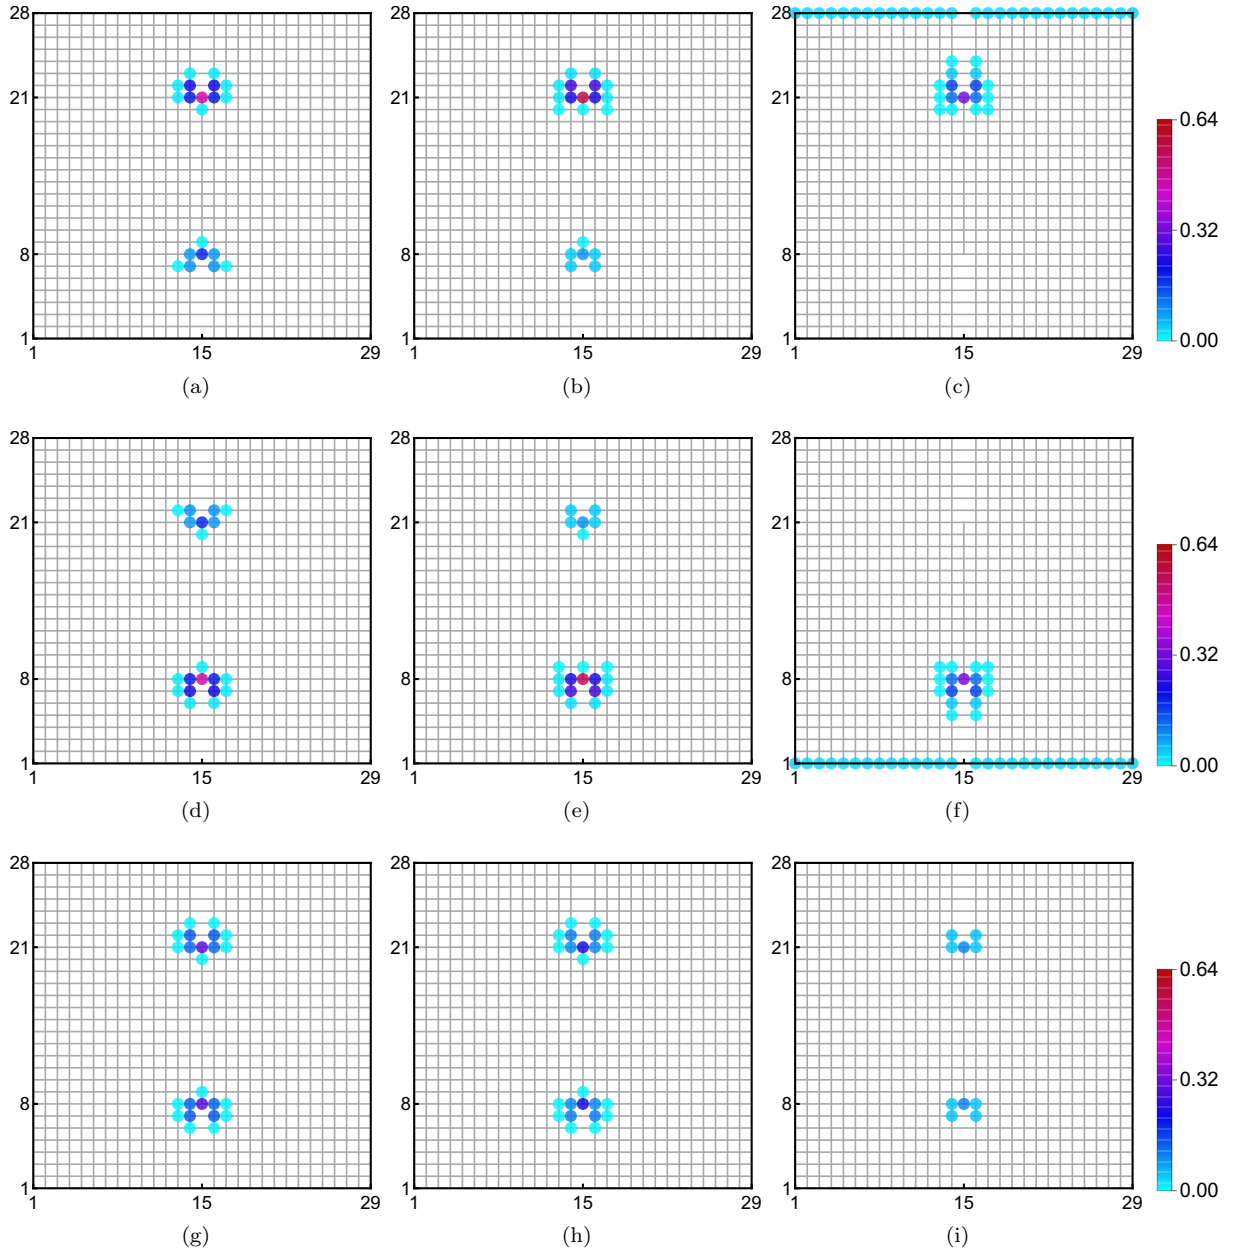

FIG. 3: Spatial profile of the density of the dislocation modes for different values of  $h_y$ , with  $m_0 = -1$ ,  $h_x = h_z = 0$ , under OBC. In (a), (b) and (c), the joint density of the right eigenvectors of the two dislocation modes is plotted for  $h_y = 0.05, 0.1$  and  $0.4$  respectively. In (d), (e) and (f), the density of the left eigenvectors is plotted for  $h_y = 0.05, 0.1$  and  $0.4$ , and in (g), (h), and (i), the biorthogonal density is plotted for  $h_y = 0.05, 0.1$  and  $0.2$ , respectively.

For the imaginary part of  $\varepsilon^2 = 0$ , we must have  $\cos k_x + \cos k_y - m_0 = 0$ . Clearly, this equation can only have a physical solution when  $|m_0| < 2$ . Then

$$\varepsilon^2 = \sin^2 k_x + \sin^2 k_y - h_z^2 = 1 - (m_0 - \cos k_y)^2 + \sin^2 k_y - h_z^2 = 2 - m_0^2 + \underbrace{2m_0 \cos k_y - 2 \cos^2 k_y}_{\text{next, we analyze only this part}} - h_z^2.$$

Now,  $2m_0 \cos k_y - 2 \cos^2 k_y = 2(\frac{m_0^2}{4} - (\cos k_y - \frac{m_0}{2})^2)$ . Let us only focus on the case  $-2 < m_0 < 0$ , which hosts dislocation modes. Here we must have  $-1 < \cos k_y < (m_0 + 1)$ , for magnitude of  $\cos k_x$  to be less than 1. The points  $-1$  and  $(m_0 + 1)$  are equally apart from  $\frac{m_0}{2}$ , and the minimum of  $2(\frac{m_0^2}{4} - (\cos k_y - \frac{m_0}{2})^2)$  is obtained at  $\cos k_y = -1$

or  $(m_0 + 1)$ , and the minimum value is  $-2m_0 - 2$ . Then,  $\varepsilon^2 > -2m_0 - m_0^2 - h_z^2$ . Thus, we get,  $h_z^* = \sqrt{-2m_0 - m_0^2}$ , which is plotted in Fig. 2(b) of the main paper. For  $0 < m_0 < 2$ , it can be shown that  $h_z^* = \sqrt{2m_0 - m_0^2}$ . Combining the two cases, we get  $h_z^* = \sqrt{2|m_0| - m_0^2}$ . The exceptional points appear at  $\cos k_x = \cos k_y = \frac{m_0}{2}$ .

## V. TOPOLOGICAL INVARIANT: CHERN NUMBER

The Hermitian Chern insulator can be identified with a topological invariant, the Chern number. The corresponding Berry Curvature is defined as

$$\Omega(\mathbf{k}) = i \left( \left\langle \frac{\partial}{\partial k_x} \psi(\mathbf{k}) \left| \frac{\partial}{\partial k_y} \psi(\mathbf{k}) \right\rangle - \left\langle \frac{\partial}{\partial k_y} \psi(\mathbf{k}) \left| \frac{\partial}{\partial k_x} \psi(\mathbf{k}) \right\rangle \right), \quad (17)$$

where  $|\psi(\mathbf{k})\rangle$  is the negative energy eigenket of the Hamiltonian from Eq. (1) when  $h_\mu = 0$ . The Chern number ( $C$ ) is then defined as the integral of the Berry curvature over the 1st Brillouin Zone (BZ), with a factor of  $\frac{1}{2\pi}$

$$C = \frac{1}{2\pi} \int_{(k_x, k_y) \in \text{BZ}} \Omega(\mathbf{k}) d^2 \mathbf{k} \quad (18)$$

In the model we have taken, for  $-2 < m_0 < 0$ , the Chern number is  $-1$ , while for  $0 < m_0 < 2$ , the Chern number is  $+1$ , and it is 0 for  $|m_0| > 2$ . The same value of Chern number continues to hold as we introduce non-Hermitian parameters  $h_x, h_y$  and  $h_z$ , until we reach an exceptional point [1].

For a non-Hermitian system, we have both the left and right eigenvectors, and there are four choices for defining the corresponding Berry Curvature

$$\Omega_{\text{NH}}(\mathbf{k}) = i \left( \left\langle \frac{\partial}{\partial k_x} \chi(\mathbf{k}) \left| \frac{\partial}{\partial k_y} \psi(\mathbf{k}) \right\rangle - \left\langle \frac{\partial}{\partial k_y} \chi(\mathbf{k}) \left| \frac{\partial}{\partial k_x} \psi(\mathbf{k}) \right\rangle \right), \quad (19)$$

where  $|\chi(\mathbf{k})\rangle$  and  $|\psi(\mathbf{k})\rangle$  can be either of  $|\psi\rangle_{R,L}$  [1, 2]. It has been shown in Ref. [3] that all the four choices lead to the same Chern number.

In this paper, we utilized a different method to calculate the Chern Number. For a Hermitian Chern Insulator, if the Hamiltonian is defined as  $\mathcal{H}(\mathbf{k}) = \mathbf{d}(\mathbf{k}) \cdot \boldsymbol{\sigma}$ , then the Berry Curvature is given by [4]

$$\Omega(\mathbf{k}) = \frac{1}{2} \hat{\mathbf{d}}(\mathbf{k}) \cdot \left( \frac{\partial \hat{\mathbf{d}}(\mathbf{k})}{\partial k_x} \times \frac{\partial \hat{\mathbf{d}}(\mathbf{k})}{\partial k_y} \right), \quad (20)$$

where  $\hat{\mathbf{d}}(\mathbf{k}) = \frac{\mathbf{d}(\mathbf{k})}{\sqrt{d_x(\mathbf{k})^2 + d_y(\mathbf{k})^2 + d_z(\mathbf{k})^2}}$ . We took the non-Hermitian operator from Eq. (1), and generalized the above relation to calculate the non-Hermitian Chern number, given by

$$C_{\text{NH}} = \text{Re} \int_{(k_x, k_y) \in \text{BZ}} \frac{d^2 \mathbf{k}}{4\pi} \left[ \hat{\mathbf{d}}_{\text{NH}}(\mathbf{k}) \cdot \left( \frac{\partial \hat{\mathbf{d}}_{\text{NH}}(\mathbf{k})}{\partial k_x} \times \frac{\partial \hat{\mathbf{d}}_{\text{NH}}(\mathbf{k})}{\partial k_y} \right) \right], \quad (21)$$

with  $\mathbf{d}_{\text{NH}}(\mathbf{k}) = \mathbf{d}(\mathbf{k}) + \mathbf{h}$ . We found that the non-Hermitian Chern number calculated with this formula agrees with that in Ref. [1]. Dislocation modes are observed in the regime  $C_{\text{NH}} = -1$ .

## VI. DENSITY OF DISLOCATION MODES UNDER OPEN BOUNDARY CONDITION

While we can theoretically study systems under periodic boundary condition (PBC), an experimental sample would usually have open boundary condition (OBC). When no dislocation is present, under OBC, the non-Hermitian systems show skin effect, where the density of a macroscopic number of states shift to the boundary of the system. When dislocation is present, the system initially shows dislocation modes that are highly localized near their cores.

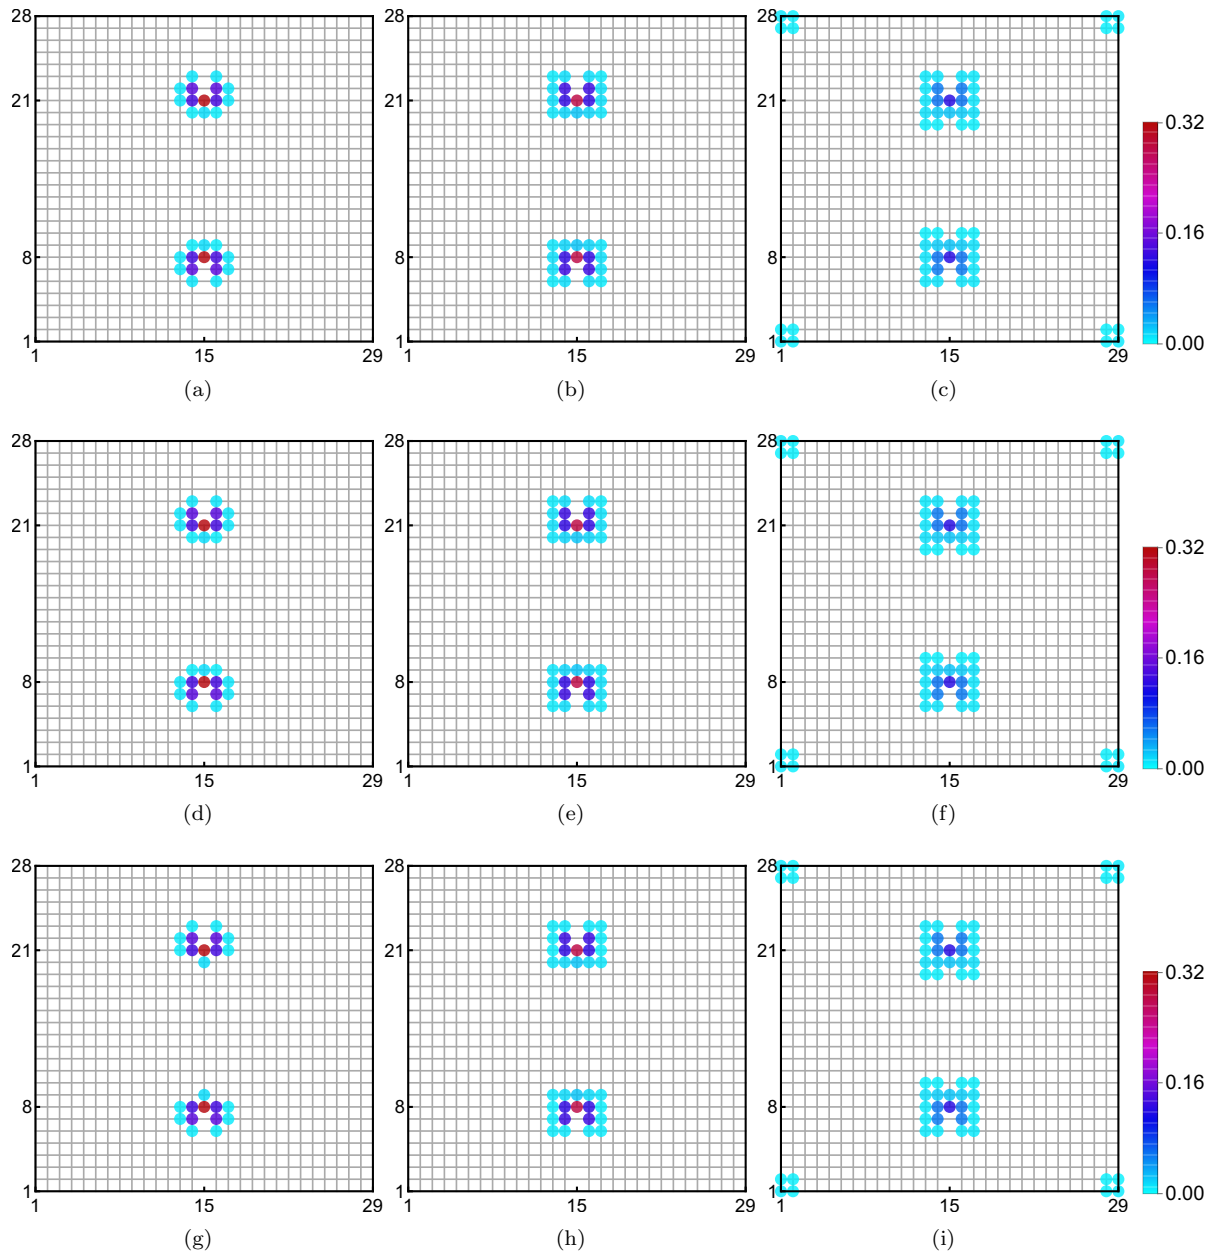

FIG. 4: Spatial profile of the density of the dislocation mode for different values of  $h_z$ , with  $m_0 = -1$ ,  $h_x = h_y = 0$ , under OBC. In (a), (b) and (c), the joint density of the right eigenvectors of the two dislocation modes is plotted for  $h_z = 0.2, 0.4$  and  $0.7$  respectively. In (d), (e) and (f), the density of the left eigenvectors is plotted for the same set of values of  $h_z$ , and in (g), (h), and (i), the biorthogonal density is plotted. In Fig. (c), (f) and (i), the dislocation modes gradually shift predominantly to the four corners of the system, maintaining the  $C_4$  symmetry.

But as we increase the non-Hermitian parameters ( $h_x, h_y, h_z$ ), the system gradually begins to show skin effect (at a value of  $h_{x,y,z} < h_{x,y,z}^*$ ), after which no dislocation modes are found anymore. While under PBC, dislocation modes are always present until  $h_{x,y,z} = h_{x,y,z}^*$ .

The spatial profile of the density of the dilocation modes of different values of  $h_x, h_y$  and  $h_z$  are plotted in Fig. 2, Fig. 3 and Fig. 4, respectively. In the rightmost column of each figure, the shift from a dislocation mode to the skin effect can be seen.

## VII. CODE FOR NUMERICAL CALCULATION

The numerical calculation was primarily performed in GNU Octave [5], and the code is available at GitHub [6].

- 
- [1] K. Kawabata, K. Shiozaki, and M. Ueda, Phys. Rev. B **98**, 165148 (2018).
  - [2] S-D Liang and G-Y Huang, Phys. Rev. A **87**, 012118 (2013).
  - [3] H. Shen, B. Zhen, and L. Fu, Phys. Rev. Lett. **120**, 146402 (2018).
  - [4] R. Shankar, arXiv:1804.06471 (2018).
  - [5] J. W. Eaton, D. Bateman, S. Hauberg, R. Wehbring, *GNU Octave version 5.2.0 manual: a high-level interactive language for numerical computations* (2019). <https://www.gnu.org/software/octave/doc/v5.2.0/>
  - [6] A. Panigrahi, Codes for Non-Hermitian dislocation modes: Stability and melting across exceptional points (2021). <https://github.com/apandada1/NHDislocQAH1>
